# Supplementary material for: Ground-state phase diagram of the three-band Hubbard model from density matrix embedding theory
Source: arXiv:2001.04951 ancillary file (2020-11-30)
Supplement: Supplementary file 1 [file Supplemental-Material-Three-Band-Hub-DMET.pdf]

# Supplemental Material to "Ground-state phase diagram of the three-band Hubbard model from density matrix embedding theory"

Zhi-Hao Cui,[1] Chong Sun,[1] Ushnish Ray,[1] Bo-Xiao Zheng,[2,1,3] Qiming Sun,[2,1] and Garnet Kin-Lic Chan[1,*]

[1]*Division of Chemistry and Chemical Engineering, California Institute of Technology, Pasadena, California 91125, United States*
[2]*AxiomQuant Investment Management LLC, Shanghai 200120, China*
[3]*Department of Chemistry, Princeton University, Princeton, New Jersey 08544, United States*
(Dated: October 24, 2020)

## I. DERIVATION OF EQ. (B.5) - (B.7)

We first evaluate the direct response [Eq. (B.5)]. One can expand the exponential using the interaction picture,

$$e^{\beta(h-\mu+\delta u)} = \mathcal{T}_\tau \exp\left[\int_0^\beta d\tau \delta u(\tau)\right] e^{\beta(h-\mu)}, \tag{1}$$

where $u(\tau)$ is in the interaction picture,

$$\delta u(\tau) = e^{\tau(h-\mu)} \delta u e^{-\tau(h-\mu)}. \tag{2}$$

To first order, the exponential becomes,

$$\left[1 + \int_0^\beta d\tau \delta u(\tau)\right] e^{\beta(h-\mu)}. \tag{3}$$

The density matrix is then

$$\begin{aligned}\gamma &= \left[1 + e^{\beta(h-\mu)} + \int_0^\beta d\tau \delta u(\tau)\, e^{\beta(h-\mu)}\right]^{-1} \\ &= \left\{\left(1 + e^{\beta(h-\mu)}\right)\left[1 + \left(1 + e^{\beta(h-\mu)}\right)^{-1} \int_0^\beta d\tau \delta u(\tau) e^{\beta(h-\mu)}\right]\right\}^{-1} \\ &= \left[1 + \left(1 + e^{\beta(h-\mu)}\right)^{-1} \int_0^\beta d\tau \delta u(\tau) e^{\beta(h-\mu)}\right]^{-1} \left(1 + e^{\beta(h-\mu)}\right)^{-1} \\ &= \gamma^{(0)} - \gamma^{(0)} \int_0^\beta d\tau \delta u(\tau) \gamma^{(0)} e^{\beta(h-\mu)}.\end{aligned} \tag{4}$$

We can expand the first order term in the eigenstates of $h$ (MO basis),

$$-\sum_{pq} |p\rangle \frac{1}{1 + e^{\beta(\varepsilon_p - \mu)}} \int_0^\beta d\tau e^{\tau(\varepsilon_p - \varepsilon_q)} \langle p|\delta u|q\rangle \frac{e^{\beta(\varepsilon_q - \mu)}}{1 + e^{\beta(\varepsilon_q - \mu)}} \langle q|. \tag{5}$$

Performing the integral yields

$$\sum_{pq} |p\rangle n_p \frac{1 - e^{\beta(\varepsilon_p - \varepsilon_q)}}{\varepsilon_p - \varepsilon_q} \langle p|\delta u|q\rangle (1 - n_q) \langle q|, \tag{6}$$

where $n_p \equiv 1/\left[1 + e^{\beta(\varepsilon_p - \mu)}\right]$. This expression can be easily transformed to the site basis using $|p\rangle = \sum_k |k\rangle C_{kp}$,

$$\sum_{ijklpq} |k\rangle C_{kp} n_p \frac{1 - e^{\beta(\varepsilon_p - \varepsilon_q)}}{\varepsilon_p - \varepsilon_q} C^*_{ip} \delta u_{ij} C_{jq} (1 - n_q) C^*_{lq} \langle l|, \tag{7}$$

and we finally get the derivative of the density matrix with respect to the correlation potential at a finite temperature:

$$\frac{\partial \gamma_{kl}}{\partial u_{ij}} = \sum_{pq} C_{kp} C^*_{ip} K_{pq} C_{jq} C^*_{lq}, \tag{8}$$

where

$$K_{pq} \equiv n_p (1 - n_q) \frac{1 - e^{\beta(\varepsilon_p - \varepsilon_q)}}{\varepsilon_p - \varepsilon_q}. \tag{9}$$

We then consider Eq. (B.7), i.e. if the Fermi level is allowed to change, this is the contribution from the change in Fermi level. The density response with respect to $\mu$, by definition, is $\frac{\partial \gamma_{kl}}{\partial \mu} = \sum_p \beta C_{kp} n_p (1 - n_p) C^*_{lp}$. The response of $\mu$ with respect to $u$ can be evaluated by taking the derivative with respect to $u_{ij}$ on both sides of the equality,

$$\sum_p \frac{1}{1 + e^{\beta(\varepsilon_p - \mu)}} = N_{\text{quasi}} \tag{10}$$

leading to the following expression,

$$\frac{\partial \mu}{\partial u_{ij}} = \left[\sum_p n_p (1 - n_p) \frac{\partial \varepsilon_p}{\partial u_{ij}}\right] \Big/ \left[\sum_p n_p (1 - n_p)\right] \tag{11}$$

By using the first order perturbation expression for the orbital energy, we reach the final expression for the $\mu$ contribution,

$$\frac{\partial \mu}{\partial u_{ij}} = \left[\sum_p n_p (1 - n_p) C^*_{ip} C_{jp}\right] \Big/ \left[\sum_p n_p (1 - n_p)\right]. \tag{12}$$

## II. ANTIFERROMAGNETIC ORDER OF ONE-BAND HUBBARD MODEL

See Fig. S1 for the AFM order of the one-band Hubbard model from DMET with different cluster sizes.

## III. PHASE DIAGRAM OF HYBERTSEN AND MARTIN MODELS

See Fig. S2 for the antiferromagnetic (AFM) and superconducting (SC) order of the three-band Hubbard model with Hybertsen and Martin minimal parametrizations from DMET.

* gkc1000@gmail.com

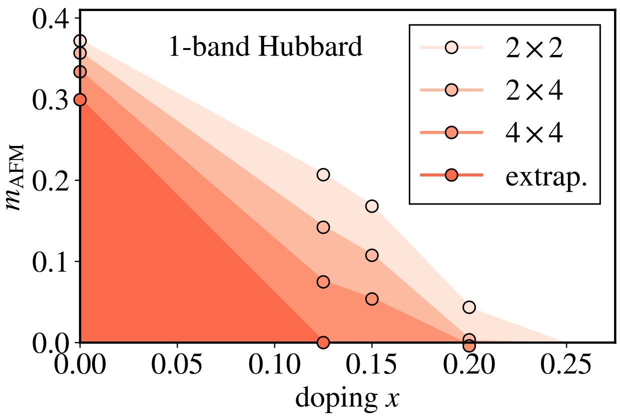


FIG. S1: AFM order parameter of the doped one-band Hubbard model ($U = 6$) from DMET with different cluster sizes ($2 \times 2$, $2 \times 4$ and $4 \times 4$) and the corresponding extrapolated value. The data are taken from Ref. [1].

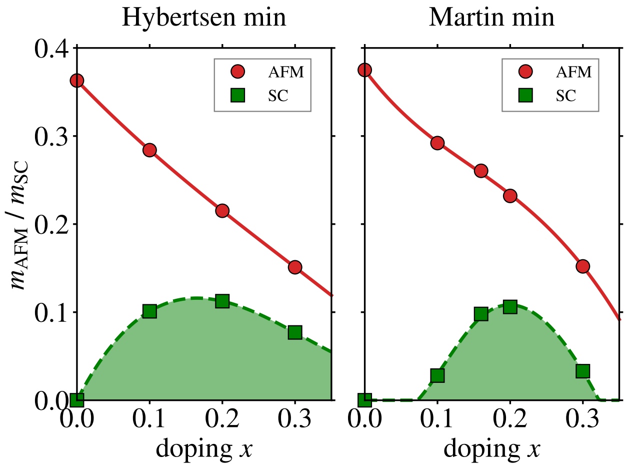


FIG. S2: AFM and SC order parameter of the hole-doped three-band Hubbard model (Hybertsen and Martin parameter sets) from DMET.

## IV. CHARGE, SPIN AND PAIRING ORDERS AT DIFFERENT DOPINGS AND PARAMETRIZATIONS

See Fig. S3 - S8 for charge, spin and pairing patterns at different dopings and parametrizations of the three-band Hubbard model.

[1] B.-X. Zheng and G. K.-L. Chan, Ground-state phase diagram of the square lattice Hubbard model from density matrix embedding theory, Phys. Rev. B **93**, 035126 (2016).

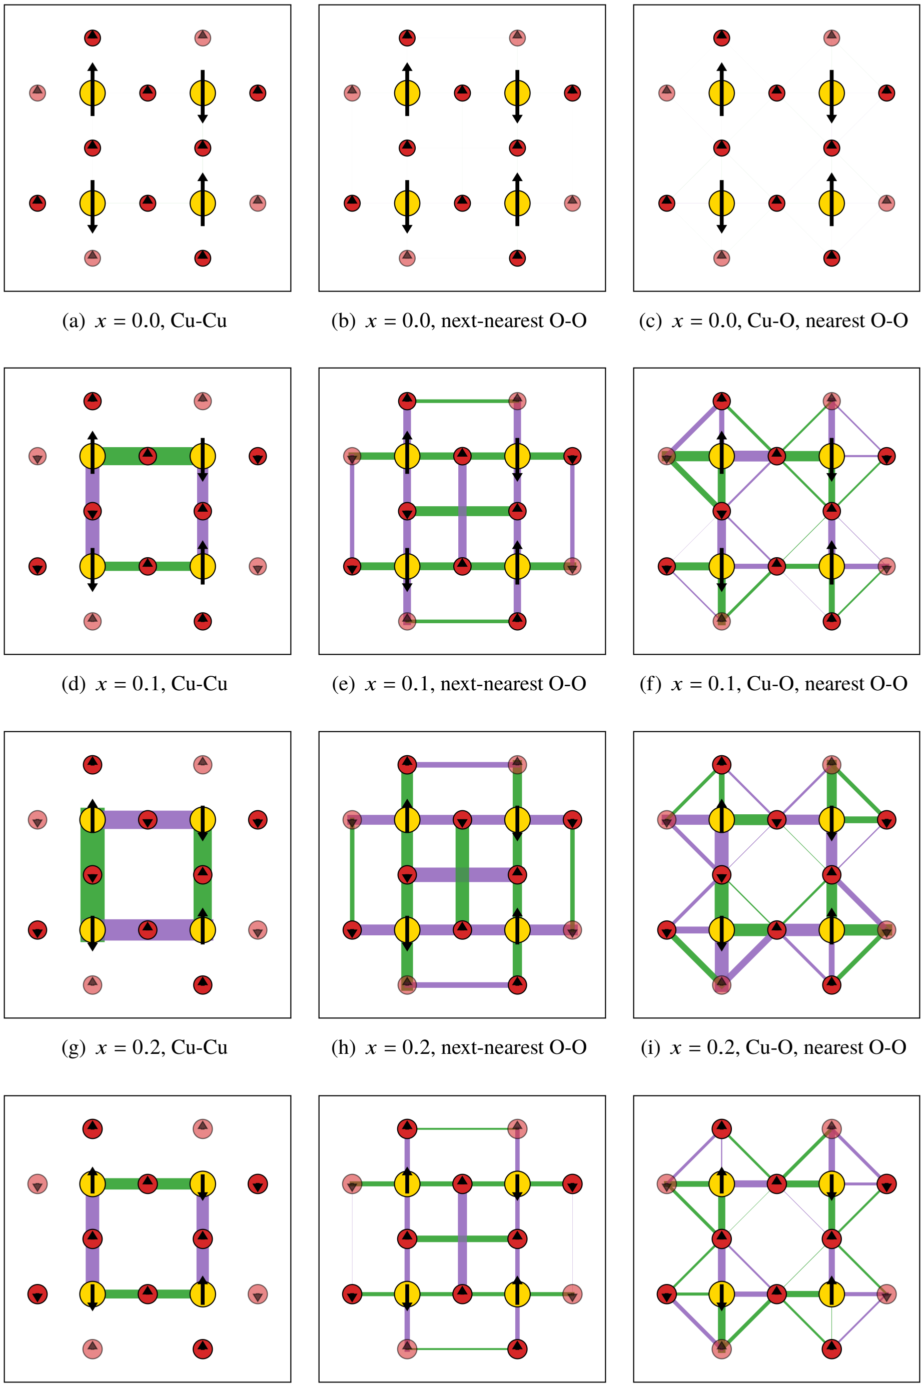

(a) $x$ = 0.0, Cu-Cu (b) $x$ = 0.0, next-nearest O-O (c) $x$ = 0.0, Cu-O, nearest O-O

(d) $x$ = 0.1, Cu-Cu (e) $x$ = 0.1, next-nearest O-O (f) $x$ = 0.1, Cu-O, nearest O-O

(g) $x$ = 0.2, Cu-Cu (h) $x$ = 0.2, next-nearest O-O (i) $x$ = 0.2, Cu-O, nearest O-O

(j) $x$ = 0.3, Cu-Cu (k) $x$ = 0.3, next-nearest O-O (l) $x$ = 0.3, Cu-O, nearest O-O

FIG. S3: Charge, spin and pairing patterns for the hole-doped Hybertsen model. See the caption of Fig. 9 in the main text for details.

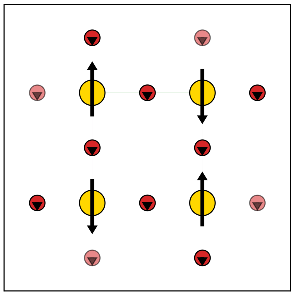

(a) $x$ = 0.0, Cu-Cu

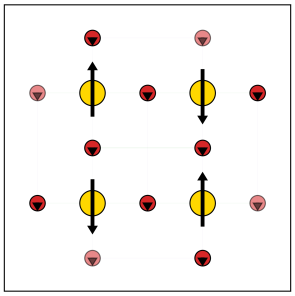

(b) $x$ = 0.0, next-nearest O-O

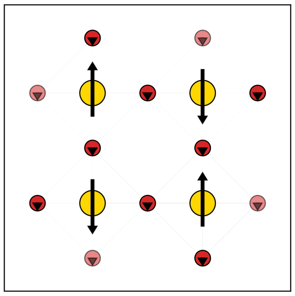

(c) $x$ = 0.0, Cu-O, nearest O-O

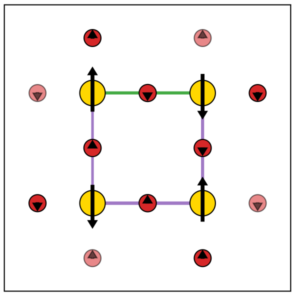

(d) $x$ = 0.1, Cu-Cu

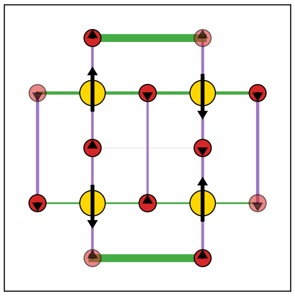

(e) $x$ = 0.1, next-nearest O-O

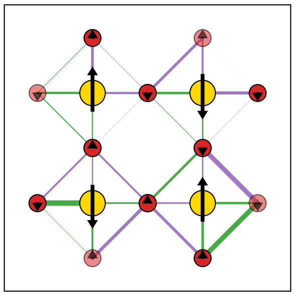

(f) $x$ = 0.1, Cu-O, nearest O-O

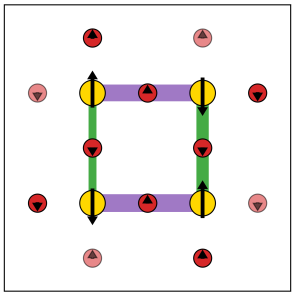

(g) $x$ = 0.2, Cu-Cu

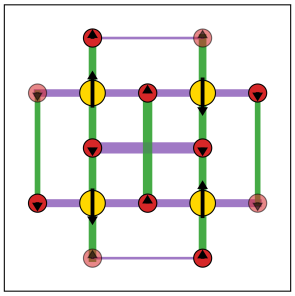

(h) $x$ = 0.2, next-nearest O-O

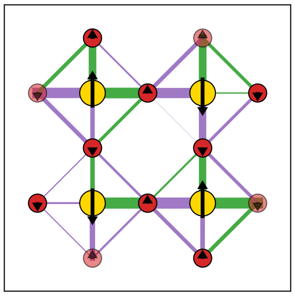

(i) $x$ = 0.2, Cu-O, nearest O-O

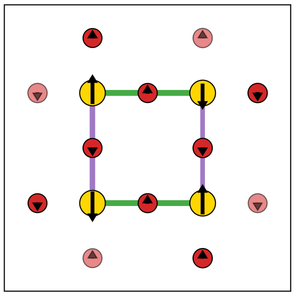

(j) $x$ = 0.3, Cu-Cu

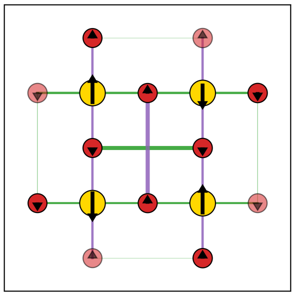

(k) $x$ = 0.3, next-nearest O-O

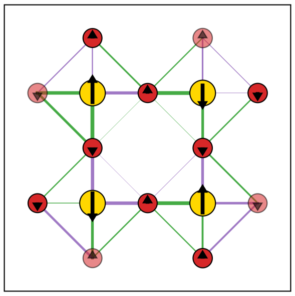

(l) $x$ = 0.3, Cu-O, nearest O-O

FIG. S4: Charge, spin and pairing distributions of the hole-doped Martin model. See the caption of Fig. 9 in the main text for details.

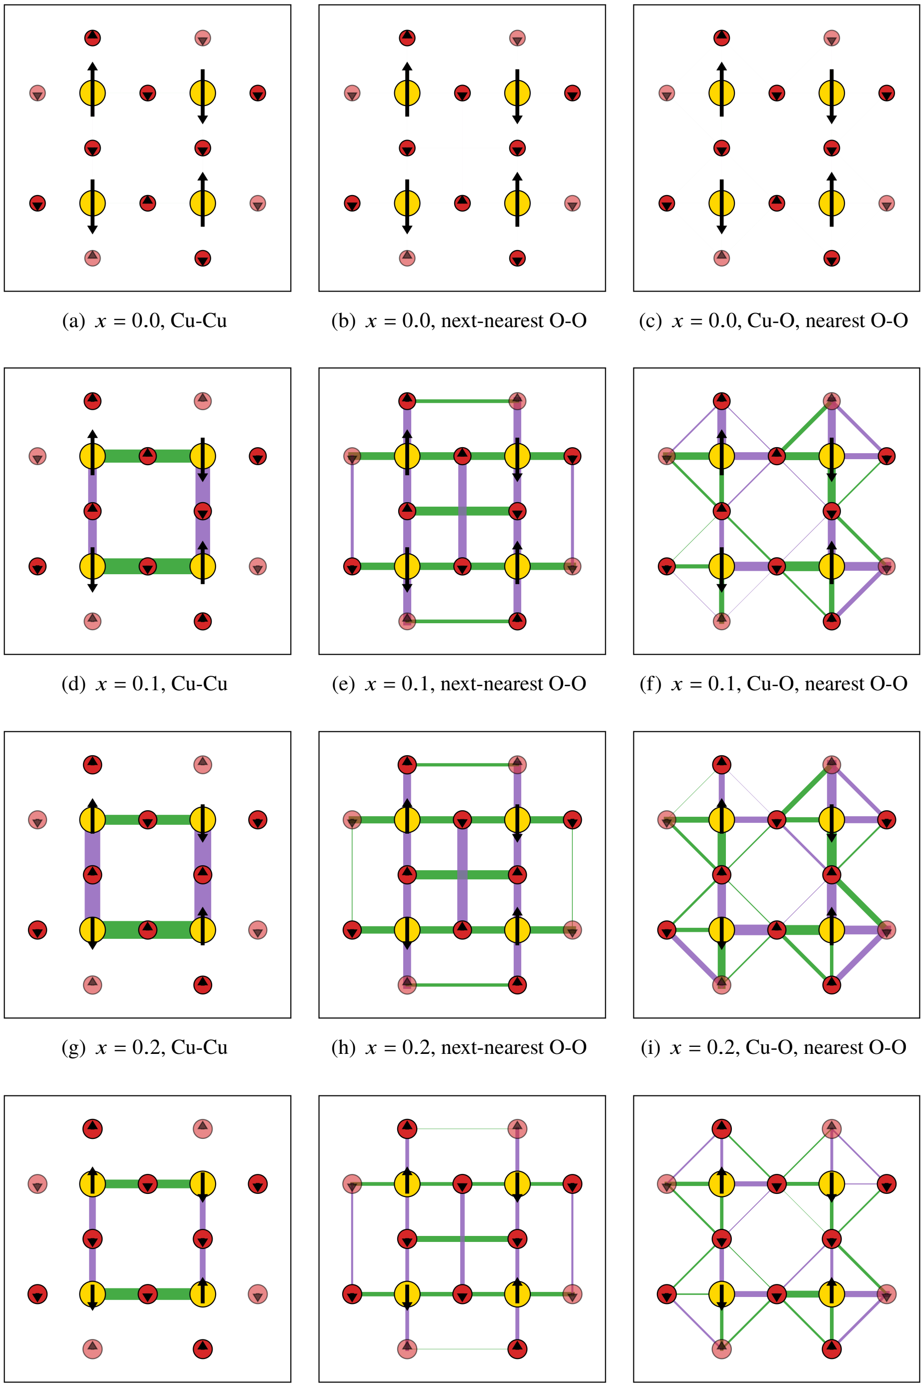

(a) $x = 0.0$, Cu-Cu (b) $x = 0.0$, next-nearest O-O (c) $x = 0.0$, Cu-O, nearest O-O

(d) $x = 0.1$, Cu-Cu (e) $x = 0.1$, next-nearest O-O (f) $x = 0.1$, Cu-O, nearest O-O

(g) $x = 0.2$, Cu-Cu (h) $x = 0.2$, next-nearest O-O (i) $x = 0.2$, Cu-O, nearest O-O

(j) $x = 0.3$, Cu-Cu (k) $x = 0.3$, next-nearest O-O (l) $x = 0.3$, Cu-O, nearest O-O

FIG. S5: Charge, spin and pairing distributions of the Hanke minimal model. See the caption of Fig. 9 in the main text for details.

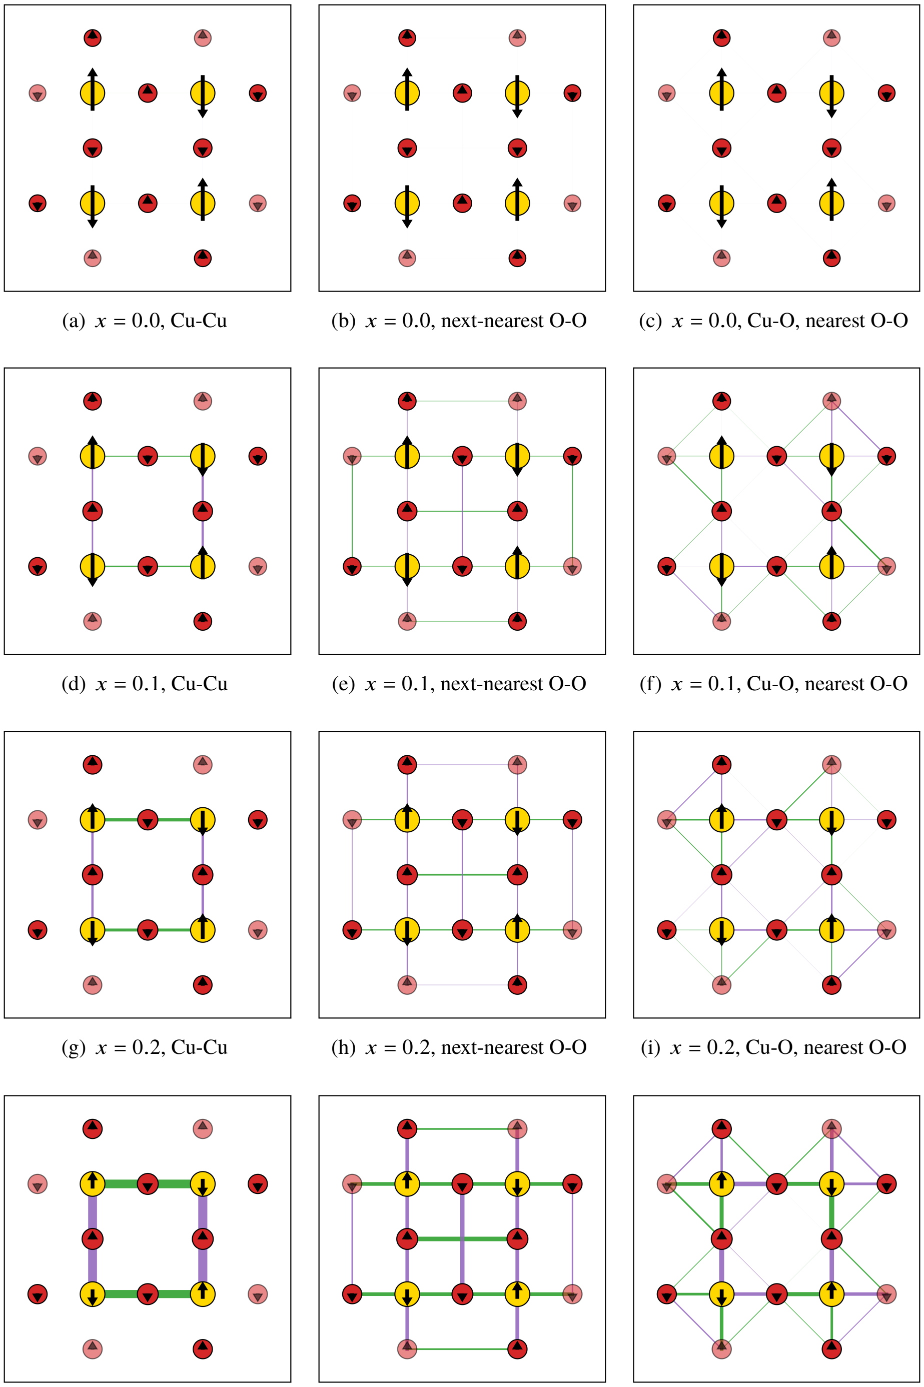

(a) $x$ = 0.0, Cu-Cu (b) $x$ = 0.0, next-nearest O-O (c) $x$ = 0.0, Cu-O, nearest O-O

(d) $x$ = 0.1, Cu-Cu (e) $x$ = 0.1, next-nearest O-O (f) $x$ = 0.1, Cu-O, nearest O-O

(g) $x$ = 0.2, Cu-Cu (h) $x$ = 0.2, next-nearest O-O (i) $x$ = 0.2, Cu-O, nearest O-O

(j) $x$ = 0.3, Cu-Cu (k) $x$ = 0.3, next-nearest O-O (l) $x$ = 0.3, Cu-O, nearest O-O

FIG. S6: Charge, spin and pairing distributions of the hole-doped Hanke full model (solution 2, from the strongly polarized guess). See the caption of Fig. 9 in the main text for details.

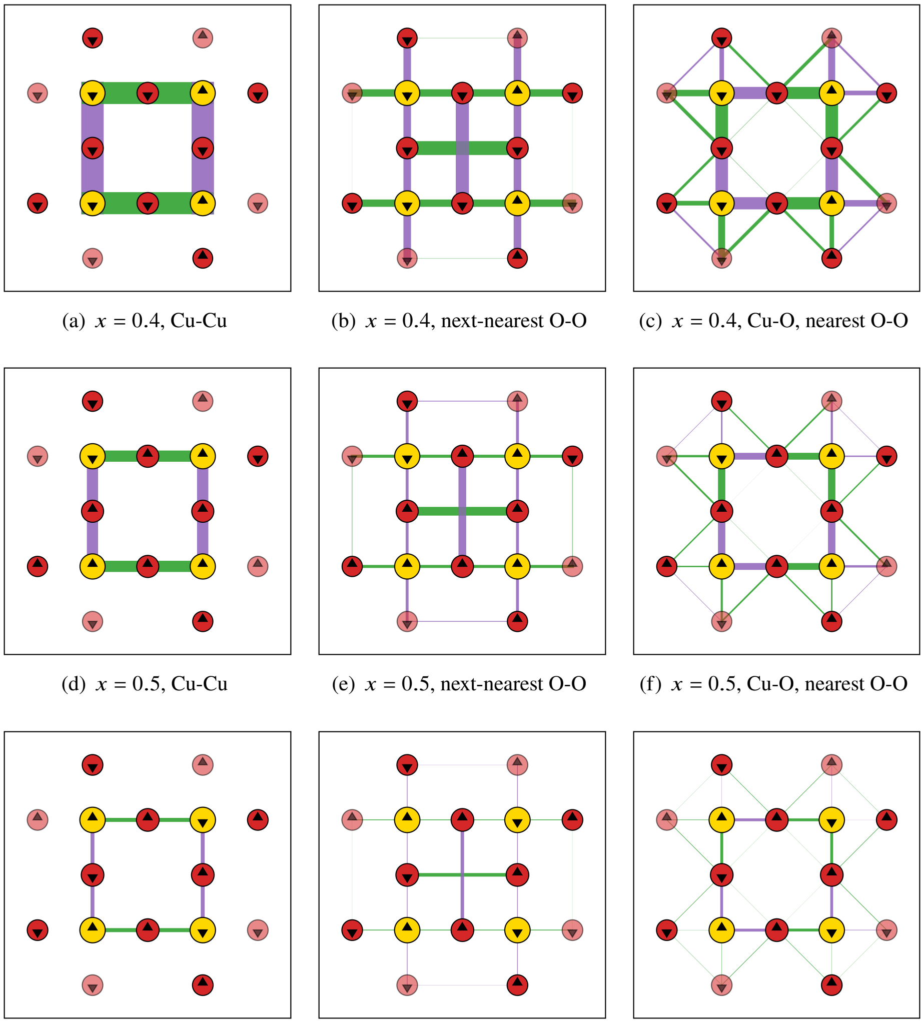

(a) $x$ = 0.4, Cu-Cu (b) $x$ = 0.4, next-nearest O-O (c) $x$ = 0.4, Cu-O, nearest O-O

(d) $x$ = 0.5, Cu-Cu (e) $x$ = 0.5, next-nearest O-O (f) $x$ = 0.5, Cu-O, nearest O-O

(g) $x$ = 0.6, Cu-Cu (h) $x$ = 0.6, next-nearest O-O (i) $x$ = 0.6, Cu-O, nearest O-O

FIG. S6: Charge, spin and pairing distributions of the hole-doped Hanke full model (solution 2, from the strongly polarized guess). See the caption of Fig. 9 in the main text for details (cont.).

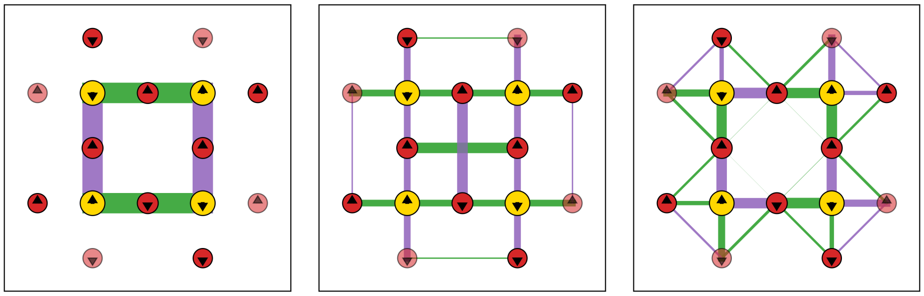

(j) $x$ = 0.3, Cu-Cu (k) $x$ = 0.3, next-nearest O-O (l) $x$ = 0.3, Cu-O, nearest O-O

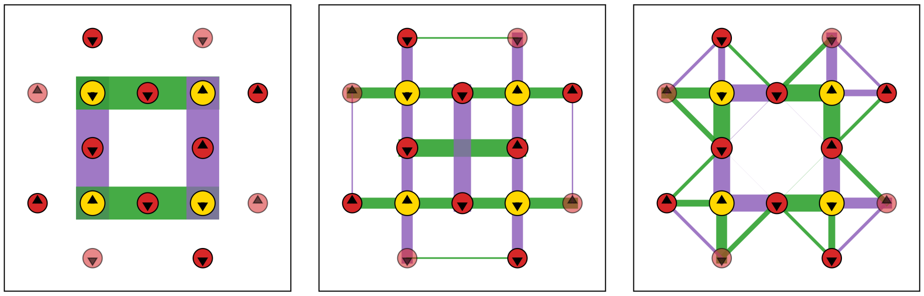

(m) $x$ = 0.31, Cu-Cu (n) $x$ = 0.31, next-nearest O-O (o) $x$ = 0.31, Cu-O, nearest O-O

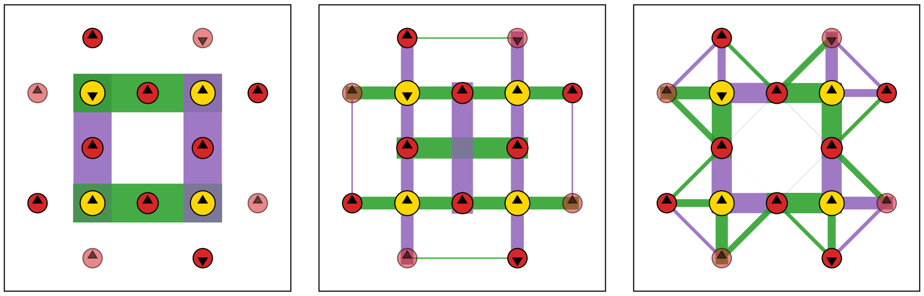

(p) $x$ = 0.325, Cu-Cu (q) $x$ = 0.325, next-nearest O-O (r) $x$ = 0.325, Cu-O, nearest O-O

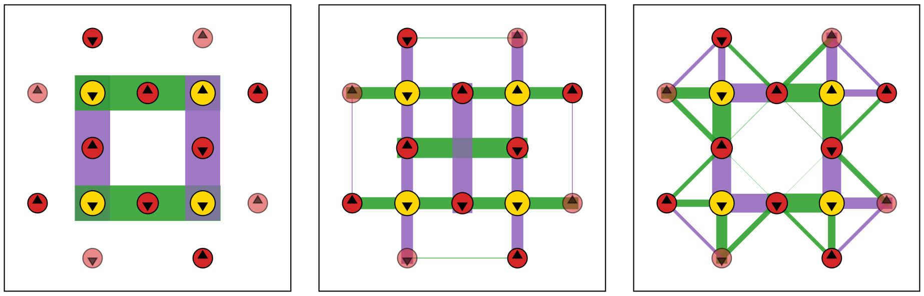

(s) $x$ = 0.35, Cu-Cu (t) $x$ = 0.35, next-nearest O-O (u) $x$ = 0.35, Cu-O, nearest O-O

FIG. S7: Charge, spin and pairing distributions of the hole-doped Hanke full model (solution 1, from the weakly polarized guess). See the caption of Fig. 9 in the main text for details.

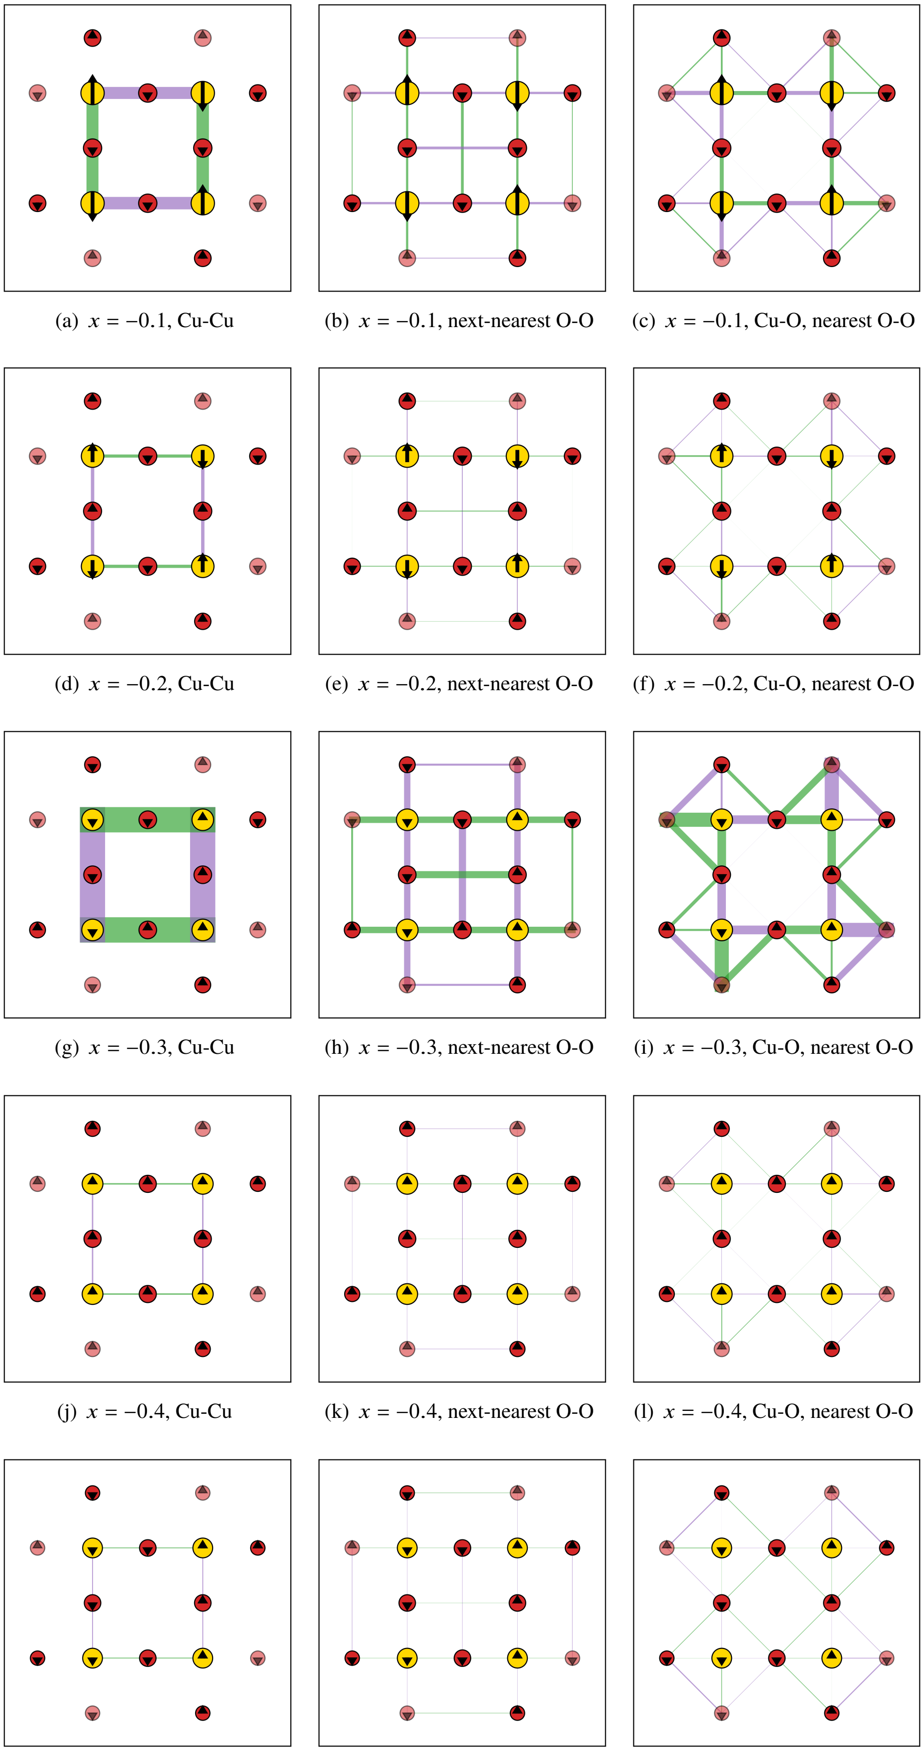

(a) $x = -0.1$, Cu-Cu (b) $x = -0.1$, next-nearest O-O (c) $x = -0.1$, Cu-O, nearest O-O

(d) $x = -0.2$, Cu-Cu (e) $x = -0.2$, next-nearest O-O (f) $x = -0.2$, Cu-O, nearest O-O

(g) $x = -0.3$, Cu-Cu (h) $x = -0.3$, next-nearest O-O (i) $x = -0.3$, Cu-O, nearest O-O

(j) $x = -0.4$, Cu-Cu (k) $x = -0.4$, next-nearest O-O (l) $x = -0.4$, Cu-O, nearest O-O

(m) $x = -0.5$, Cu-Cu (n) $x = -0.5$, next-nearest O-O (o) $x = -0.5$, Cu-O, nearest O-O

FIG. S8: Charge, spin and pairing distributions of the electron-doped Hanke full model. See the caption of Fig. 9 in the main text for details.

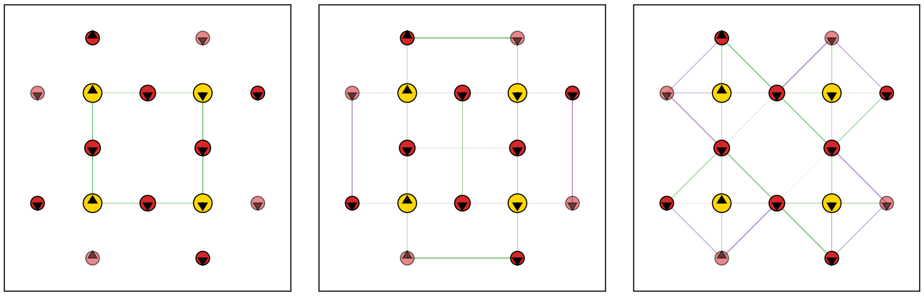

(a) $x = -0.6$, Cu-Cu (b) $x = -0.6$, next-nearest O-O (c) $x = -0.6$, Cu-O, nearest O-O

FIG. S8: Charge, spin and pairing distributions of the electron-doped Hanke full model. See the caption of Fig. 9 in the main text for details (cont.).
